# Supplementary material for: {S\textsuperscript{2}M\textsuperscript{2}}: Scalable Stereo Matching Model for Reliable Depth Estimation
Source: arXiv:2507.13229 ancillary file (2025-10-11)
Supplement: Supplementary file 1 [file supp.pdf]

# Supplementary Materials

## S<sup>2</sup>M<sup>2</sup>: Scalable Stereo Matching Model for Reliable Depth Estimation

### 1. Implementation

#### 1.1. Training Strategy

Our training methodology consists of two phases: first, establishing baseline models for our ablation studies, and second, a sequential fine-tuning process to develop our final benchmark models, which is directly built upon the first phase.

##### Phase 1: Baseline Models for Ablation Studies

The models used in our ablation studies were trained following a complete, single-stage procedure. Each model was trained on image patches of  $768 \times 448$  px with a batch size of 4 for 2,000,000 gradient updates. For optimization, we used the AdamW optimizer with a one-cycle learning rate scheduler, decaying the learning rate from an initial value of  $1 \times 10^{-5}$  to  $1 \times 10^{-6}$ .

The training was performed on a foundational set of synthetic datasets—including SceneFlow [11], TartanAir [19], and CREStereo [9]—amounting to approximately 0.5M image pairs. This process yielded our fully trained ablation models, which serve as the starting point for the next phase.

##### Phase 2: Sequential Fine-tuning for Benchmark Submission

Instead of training from scratch, our final benchmark models were developed by sequentially fine-tuning the fully trained ablation models from Phase 1. This process involves two subsequent steps:

**Step 1: Fine-tuning on an Expanded Dataset:** First, we took a converged ablation model and continued its training at the same fixed resolution ( $768 \times 448$ ). The key difference in this step was the use of a significantly expanded data pool, totaling up to 2M image pairs. This collection includes widely-used datasets in combination with additional sources such as FoundationStereo [23], IRS [18], Falling Things [17], Virtual KITTI 2 [6], DrivingStereo [28], and SMD-Net [16], among others. This step allows the model to consolidate its learned features and generalize across a much more diverse range of data distributions.

**Step 2: Multi-Resolution Fine-tuning with Gradient Checkpointing:** In the final step, the model from Step 1 was further fine-tuned across three resolutions simultaneously ( $768 \times 448$ ,  $1440 \times 1024$ , and  $1920 \times 1440$ ). This was performed on an H100×8 GPU server with a total batch size of 56.

A significant technical hurdle at this stage is the high memory requirement for high-resolution training. Processing images at  $1920 \times 1440$  px exceeds the 80GB memory capacity of a single H100 GPU. To resolve this, we employed PyTorch [13]’s gradient checkpointing feature. This technique trades computation for memory by recomputing intermediate activations during the backward pass instead of storing them all. Gradient checkpointing was essential for enabling stable, high-resolution training, allowing our final model to effectively learn features across a wide spectrum of scales.

#### 1.2. Data Augmentation

To address the practical challenges of real-world stereo matching, we employed a targeted data augmentation strategy beyond standard color and cropping adjustments [9]. Specifically, we introduce a random horizontal shift when cropping the left and right images. This technique is designed to simulate imperfect rectification and, importantly, mimic the design of benchmark datasets like Middlebury v3 [14].

In these datasets, the stereo pairs are intentionally cropped with a sample-specific horizontal offset to maximize the overlapping field of view and manage occlusions. By replicating this characteristic in our training data, our model becomes

robust to the subtle misalignments frequently present in real-world or benchmark stereo pairs. This robustness is critical for preventing performance degradation from a domain shift during testing; without it, a model trained on ideal data learns to associate strong perspective cues with large disparity values. When a test sample violates this learned correlation due to an artificial offset, the model’s predictions fail as its internal priors conflict with the ground truth.

Furthermore, a key consequence of this horizontal shift is the introduction of negative disparity values for some pixels. While unconventional, we leverage this as a deliberate training strategy. Training with these negative disparities encourages the model to learn depth relationships in a more object-centric manner. Instead of relying solely on the common assumption of positive disparity, the network is forced to more comprehensively understand the relative spatial arrangement of objects and surfaces. This, in turn, enables more flexible and accurate depth estimation, particularly around object boundaries and in scenes with complex foreground-background interactions.

## 2. Loss Function Details

The final loss function consists of four components: disparity loss, occlusion loss, confidence loss, and PMC loss, each weighted by predefined hyperparameters:

$$\mathcal{L}_{\text{total}} = \lambda_D \mathcal{L}_D + \lambda_O \mathcal{L}_O + \lambda_C \mathcal{L}_C + \lambda_{\text{PMC}} \mathcal{L}_{\text{PMC}}. \quad (1)$$

The hyperparameters are set as follows:  $\lambda_D = 1$ ,  $\lambda_O = 0.1$ ,  $\lambda_C = 0.1$ , and  $\lambda_{\text{PMC}} = 1$ . Below, we detail the disparity, occlusion, and confidence loss formulations.

### 2.1. Disparity Loss

Disparity loss supervises both the initial global disparity estimate and the refined disparities at each iteration. We use a smooth L1 loss for the initial disparity, applied only to non-occluded pixels, while the refined disparities are optimized using L1 loss over all pixels. This ensures that the network learns reliable disparity predictions across all refinement stages.

$$\mathcal{L}_D = \mathcal{L}_D^{\text{init}} + \sum_{t=1}^T \mathcal{L}_D^{(t)}, \quad (2)$$

where

$$\mathcal{L}_D^{\text{init}} = \frac{1}{|\Omega|} \sum_{(i,j) \in \Omega} \text{Smooth-}\ell_1(D_{ij}^{\text{init}}, D_{ij}^{\text{gt}}), \quad (3)$$

$$\mathcal{L}_D^{(t)} = \frac{1}{|H \times W|} \sum_{(i,j)} |D_{ij}^{(t)} - D_{ij}^{\text{gt}}|. \quad (4)$$

Here,  $\Omega = \{(i,j) \mid O(i,j) = 1\}$  is the set of non-occluded pixels, and  $H \times W$  represents all pixels in the image. The initial disparity  $D^{\text{init}}$  is supervised only on non-occluded pixels, while the refined disparities  $D^{(t)}$  (for  $t = 1, \dots, T$ ) are trained on all pixels.

### 2.2. Occlusion and Confidence Loss

The occlusion and confidence maps are learned using an L1 loss rather than binary cross-entropy to ensure numerical stability. The losses for occlusion and confidence maps follow a similar formulation:

$$\mathcal{L}_O = \mathcal{L}_O^{\text{init}} + \sum_{t=1}^T \mathcal{L}_O^{(t)}, \quad (5)$$

$$\mathcal{L}_C = \mathcal{L}_C^{\text{init}} + \sum_{t=1}^T \mathcal{L}_C^{(t)}. \quad (6)$$

Specifically, the occlusion losses are computed over all pixels:

$$\mathcal{L}_O = \frac{1}{|H \times W|} \sum_{(i,j)} |O_{ij} - O_{ij}^{\text{gt}}|. \quad (7)$$

In contrast, the initial confidence loss is computed only over non-occluded pixels, while the confidence losses in the refinement steps are optimized over all pixels:

$$\mathcal{L}_C^{\text{init}} = \frac{1}{|\Omega|} \sum_{(i,j) \in \Omega} |\Gamma_{ij}^{\text{init}} - \Gamma_{ij}^{\text{gt}}|. \quad (8)$$

$$\mathcal{L}_C^{(t)} = \frac{1}{|H \times W|} \sum_{(i,j)} |\Gamma_{ij}^{(t)} - \Gamma_{ij}^{\text{gt}}|. \quad (9)$$

Ground Truth Definition - Confidence Map ( $\Gamma$ ): Defined as 1 if the absolute disparity error is below 4 pixels, which corresponds to one pixel in the 1/4 resolution feature space; otherwise, 0.

- Occlusion Map ( $O$ ): Defined by left-right consistency check, where a pixel is non-occluded if the left-right disparity warping error is below 2 pixels.

This loss formulation ensures that occlusion and confidence estimates remain reliable throughout training while preventing numerical instability.

### 3. Synthetic Data Generation

#### 3.1. Train Dataset

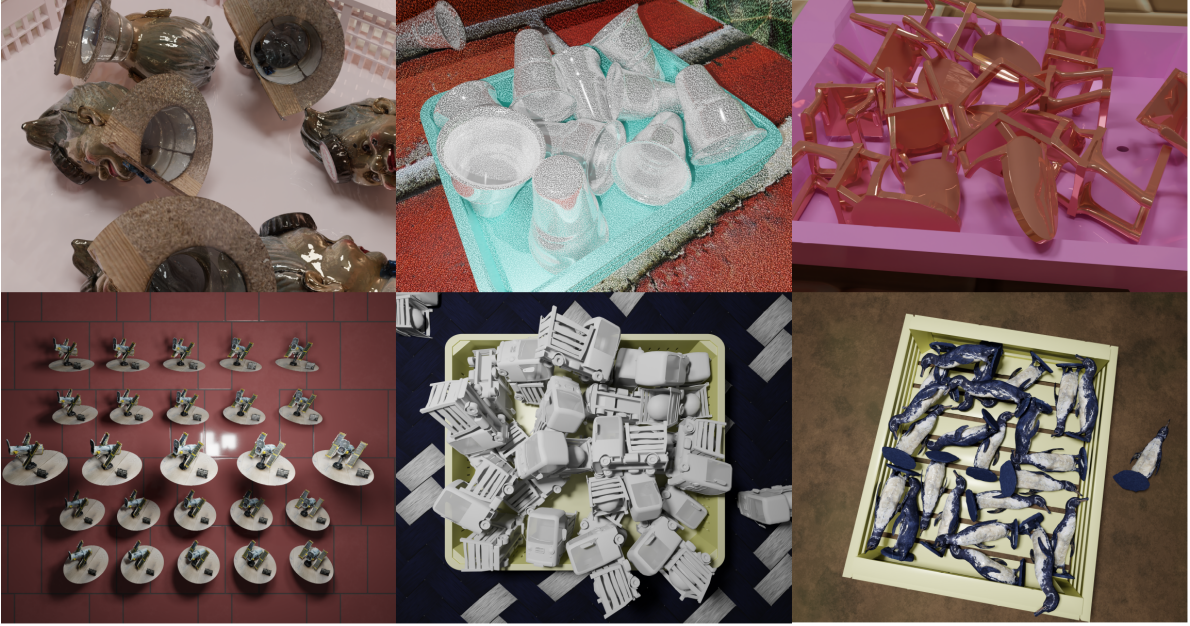

Figure 1. Configurations of scenes in our synthetic training dataset: Objects from Objaverse are randomly dropped into a bin or arranged in structured layouts, with variations in surface materials such as reflective surfaces. Some scenes also include projected random patterns to simulate active stereo scenarios.

Our basic training dataset comprises a diverse set of available synthetic datasets [6, 9, 11, 16, 17, 18, 19, 23, 28]. To further enhance the training dataset, we generated a specialized synthetic dataset to complement the existing data by leveraging 3D assets from Objaverse [4] and BlenderKit [1] within the Blender environment. The dataset was constructed through physics-based simulations where uniform object types were randomly dropped into a bin to generate realistic stacked configurations. Scenes were rendered using a stereo camera system to obtain passive RGB images, depth maps, and occlusion maps. To increase diversity, we varied object sizes, lighting conditions, bin shapes, and camera configurations. The camera was randomly positioned within the space between the top and the sides of the bin. Camera parameters were assigned random values within the following ranges for each scene generation. Field of View (FOV) was selected from 35° to 45°, and baseline was selected from 0.25m to 0.35m. The bin shape was randomly selected from a set of dozens of predefined shapes, and

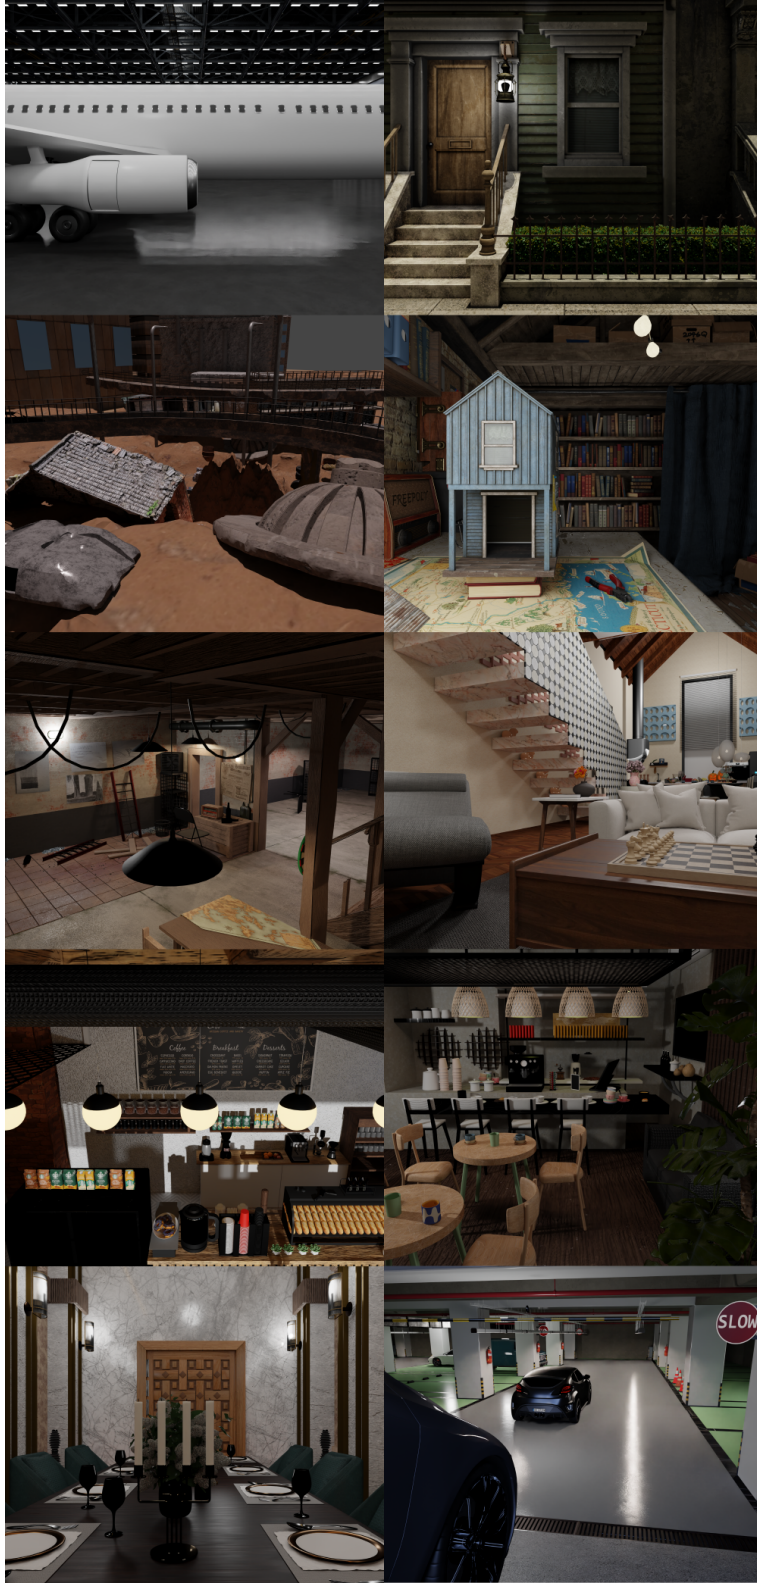

Figure 2. Configurations of scenes in our synthetic benchmark dataset: Our benchmark synthetic dataset was generated across 10 environments, encompassing indoor and outdoor settings. These include house interiors, cafes, parking lots, aircraft hangers, residential areas and abandoned urban areas, comprehensively covering various real-world spatial contexts.

its side lengths were randomly determined within the range of 0.6m to 1.2m. The materials for the floor and walls were randomly chosen from a collection of 2,176 materials provided from BlenderKit. We randomly set 2 to 5 lights assigning random values to their locations and energy. The object size was normalized such that the bounding bin volume of the object was between 10% and 20% of the bin volume. All objects within a single scene had the same size. A total of 8 to 30 objects were randomly dropped from above the bin. The scenes were rendered 3 seconds after the objects were dropped.

Additionally, we varied material properties to include challenging surface types, such as reflective and transparent materials, making the dataset more diverse and representative of real-world conditions. Alpha, roughness, and metallic values were randomly selected within the range of 0.1 to 0.7, and the index of refraction (IOR) values were randomly assigned between 1.5 and 2.5. Both the objects and the bin were designed to feature reflective and transparent surfaces.

One of the key challenges in stereo matching arises when objects exhibit repetitive structures, which can lead to ambiguities in disparity estimation. To address this, we created additional datasets containing horizontally aligned identical objects, forcing the network to learn more robust correspondences in such scenarios. Identical objects were arranged in a grid format of either 5×5 or 6×6 with uniform spacing. The objects within each horizontal row were positioned at the same height, ensuring consistent gaps between them.

Our final synthetic training dataset consists of approximately 40,000 scenes, complementing existing synthetic datasets while specifically addressing limitations such as repetitive textures, low-texture regions, and disparity ambiguities.

### 3.2. Our Synthetic Benchmark Dataset

Our benchmark dataset was constructed utilizing scenes and 3D models sourced from BlenderKit. As shown in Figure 2, the dataset comprises 10 distinct environmental categories spanning both indoor and outdoor settings under diverse illumination conditions. A total of 130 scenes were generated across these environments to address challenges in stereo depth estimation. The dataset specifically incorporates optically complex surfaces including reflective and transparent objects, horizontal repetitive structures, and scenes containing sharp depth discontinuities where distant background elements are juxtaposed with proximate foreground objects. This dataset is designed to evaluate the challenging aspects of stereo depth estimation through controlled introduction of real-world complexities.

#### 3.2.1. Analysis

Each scene in our benchmark dataset has a resolution of  $2448 \times 2048$  pixels, with stereo baselines varied between 0.1 m and 0.5 m. The disparity distribution spans from 2.19 pixels to over 1000 pixels as shown in Figure 3. Since many existing models struggle with extremely large disparity values, we performed benchmark evaluations in the following section with maximum disparity limits set at 320 pixels and 512 pixels. These limits covered 82.304% and 93.442% of the entire benchmark dataset, respectively, ensuring that the analysis remains representative of the dataset’s overall distribution.

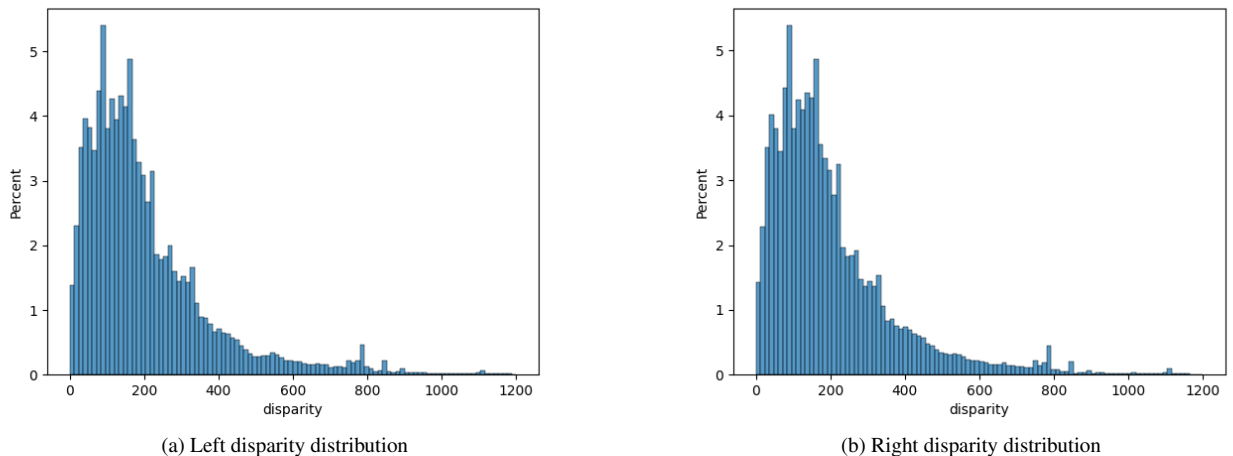

Figure 3. Benchmark dataset disparity distribution (x-axis: disparity (pixels), y-axis: proportion of the total dataset (%)): The figure illustrates the disparity distribution when the maximum disparity is set to 1200 pixels, covering 99.591% of the entire benchmark dataset.

While synthetic data generation assumes ideal stereo camera calibration, achieving perfect calibration in real-world sce-

narios is challenging, often leading to geometric misalignment. This misalignment introduces a vertical shift in the images. To rigorously examine its impact, we generated an imperfect synthetic dataset that simulates realistic calibration errors under identical conditions as the perfectly calibrated case. Instead of applying a simple vertical shift to the images, the right camera was deliberately offset perpendicular to the baseline axis by 0.4–1.8 mm during rendering, inducing physically consistent y-disparities. Across all 130 scenes, the average y-disparity measured 0.9964 pixels, with 95% of values distributed between 0.8561 and 1.1302 pixels per scene (Table 1).

|                | y-disparity                 |
|----------------|-----------------------------|
| <b>Average</b> | 0.8561 pixel - 1.1302 pixel |
| <b>Minimum</b> | 0.0132 pixel - 0.6887 pixel |
| <b>Maximum</b> | 0.8561 pixel - 9.9977 pixel |

Table 1. Y-disparity analysis on imperfect calibration dataset with value range for 95%

#### 4. Critical Analysis of Fine-Tuning Effects on the KITTI Benchmark

While fine-tuning on the KITTI dataset [7, 12] is a common practice to boost benchmark scores, its impact on a model’s true generalization capability warrants a deeper investigation. In this section, we present additional experiments arguing that the observed improvements in error metrics after fine-tuning may not represent a genuine enhancement in stereo accuracy, but rather an overfitting to the inherent noise and systematic biases present in the LiDAR-derived ground truth. Specifically, the noise often originates from the LiDAR sensor’s own physical limitations, while the systematic biases can be traced to more structured issues, such as spatio-temporal misalignments caused by moving vehicles or subtle calibration errors between the stereo rig and the LiDAR sensor.

##### Quantitative Analysis: Contradiction in Metrics

Our initial analysis begins with a quantitative comparison of our model before and after fine-tuning on the KITTI 2015 [12] training set. As shown in Table 2, fine-tuning leads to a significant reduction in standard error metrics such as End-Point-Error (EPE) and Bad-2.0 on the training data.

However, this apparent improvement is contradicted by a notable decrease in photometric consistency, which we measure using the Structural Similarity Index (SSIM) [21]. To calculate SSIM, we warp the right image to the left view’s perspective using the estimated disparity map and measure their similarity. This comparison was performed exclusively on non-occluded regions, which are identified using a predicted occlusion map from the model. While we acknowledge that SSIM is not a perfect representation of photometric consistency due to the presence of non-Lambertian surfaces (e.g., reflections), a strong positive correlation between improvements in error metrics and photometric consistency is typically expected. The observed divergence—where disparity metrics improve while SSIM deteriorates—is a strong indication of an underlying issue with the fine-tuning process. It strongly suggests that the fine-tuned model is producing disparity maps that are less geometrically consistent with the scene, potentially by overfitting to artifacts in the ground truth labels rather than reconstructing the true scene structure. This effect has also been observed in other works [29], where fine-tuning on specific real-world datasets degraded performance on other domains.

| Fine Tuning | Split | EPE   | Bad-2.0 | SSIM           |
|-------------|-------|-------|---------|----------------|
| No          | Train | 0.885 | 1.100   | 0.883 (-)      |
| Yes         | Train | 0.461 | 0.280   | 0.840 (↓0.043) |
| No          | Test  | -     | -       | 0.879 (-)      |
| Yes         | Test  | -     | -       | 0.844 (↓0.035) |

Table 2. Impact of fine-tuning on the KITTI 2015 training and test sets. While fine-tuning significantly improves disparity accuracy metrics (EPE, Bad-2.0) on the training set, the photometric consistency (SSIM) decreases on both training and test sets. This suggests potential overfitting to dataset-specific noise and a reduction in generalization.

##### Qualitative Inspection: Evidence of Ground Truth Bias

To understand the source of this metric-consistency discrepancy, we performed detailed 3D visualizations and manual inspections of the disparity maps. We conducted a comprehensive comparison across three different architectures:

- **Our Model( $S^2M^2$ )**, evaluated in both its zero-shot and fine-tuned states.
- **Selective-IGEV** [20], also evaluated in its zero-shot and fine-tuned states.
- **FoundationStereo** [23], evaluated in its zero-shot configuration.

Our investigation revealed a consistent trend among all three zero-shot models, as visualized in Figure 4. Our model and FoundationStereo [23] produced disparity maps that, when visualized as 3D point clouds, were structurally sound, visually clean, and highly consistent with the image content. The zero-shot output from Selective-IGEV [20], albeit with slightly lower visual quality, was broadly consistent with this finding.

Crucially, we observed spatially varying biases between the outputs of all these zero-shot models and the provided KITTI ground truth. We manually verified biases in areas with clear geometric features, such as the sharp, well-defined edges of vehicle license plates, where our inspection confirmed that the ground truth disparity exhibits a bias of up to 2 pixels compared to our manually calculated values.

In contrast, the fine-tuned versions of both our model and Selective-IGEV exhibited the same clear signs of adapting to this ground truth noise. These models produce disparity maps with blurry edges and structures that, while numerically closer to the noisy ground truth, are less consistent with the actual image content. This demonstrates that the models have effectively learned to replicate the dataset’s inherent bias.

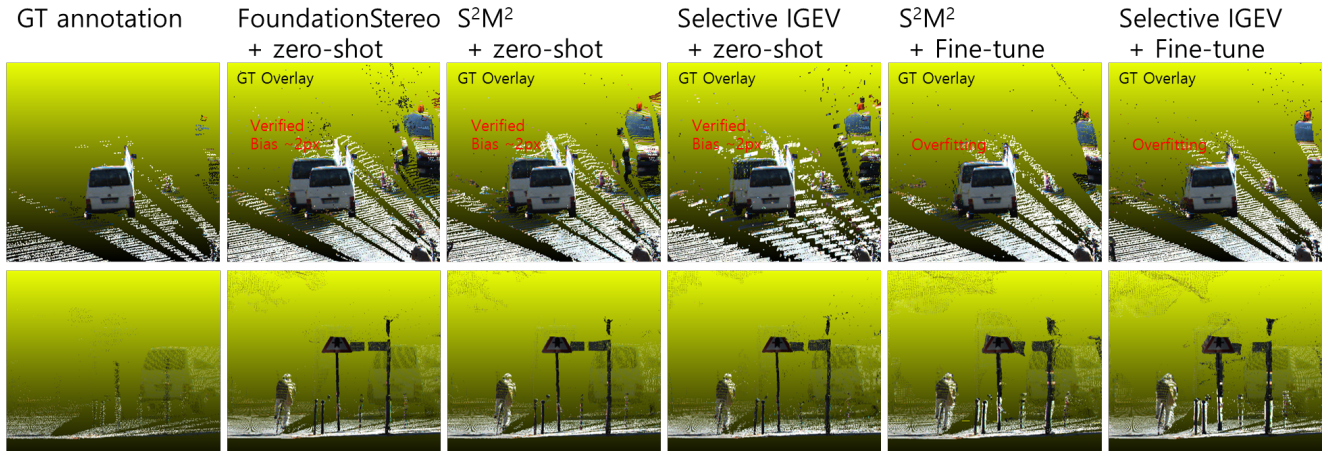

Figure 4. Qualitative comparison illustrating the negative effects of fine-tuning on a KITTI 2015 sample. **Top row:** Focuses on a vehicle area to highlight the bias between the zero-shot and fine-tuned models. The ground truth annotation from the training data is overlaid to visualize how the fine-tuned model adapts to the noisy label. **Bottom row:** Shows a pillar structure where the fine-tuned model estimates the pillar to be significantly thicker than its actual structure, a distortion not present in the zero-shot output.

The combined quantitative and qualitative evidence strongly suggests that the numerical improvements from fine-tuning on KITTI are deceptive. The models are effectively learning the noise and systematic biases of the LiDAR-derived ground truth. The concurrent drop in photometric consistency (SSIM) and the qualitative evidence of fitting to noisy labels indicate that this fine-tuning process harms the model’s generalization capabilities, even as it achieves a lower error score on the benchmark’s training set.

## 5. Comprehensive Analysis on Our Synthetic Benchmark

To gain deeper insight into the capabilities and limitations of stereo matching models, we conducted a comprehensive analysis on our synthetic benchmark. We investigate model robustness by systematically evaluating the impact of three key factors: **stereo calibration quality**, **input image resolution**, and **maximum disparity range**. In the following sections, we vary one factor at a time to isolate its effect on model accuracy and robustness. Our analysis also examines the trade-off between accuracy and processing speed, offering a thorough assessment of model efficiency under different conditions.

We benchmarked a total of 16 models, including three variants of  $S^2M^2$ , on a single NVIDIA H100 GPU with 80GB of VRAM. To ensure a fair comparison, we adhered to the hyperparameter configurations and refinement iterations proposed in each model’s original publication. Furthermore, our synthetic data contains unreliable values in regions of large depth, which correspond to small disparity values. To mitigate the impact of this, we excluded disparities below 10 from our evaluation metrics.

### 5.1. Analysis of Calibration Error Impact

As expected, the introduction of stereo calibration errors results in a performance decrease across all benchmarked models. However, the magnitude of this degradation is not uniform across the board. As illustrated in Figure 5, we observed a particularly severe drop in accuracy for models designed to be lightweight. For instance, models such as FastACV [26] and CoEx [2] exhibited a more pronounced performance decline compared to more robust, heavier architectures. This finding highlights a critical trade-off: while lightweight models provide computational efficiency, they may lack resilience to the inevitable calibration imperfections found in real-world scenarios.

### 5.2. Analysis of Input Resolution Impact

Ideally, higher input resolution should lead to more accurate disparity predictions. However, our analysis reveals that this is not universally the case. To investigate this, we evaluated all models by combining two resolutions (full, half) with two maximum disparity settings ( $D_{max} = 320$  and  $D_{max} = 960$ ). The results, plotted as accuracy versus processing speed, are presented in Figure 6 and Figure 7.

As expected, all models run significantly faster at half resolution. A distinct trend was observed in lightweight models, which not only gained speed but also often achieved superior accuracy at half resolution, especially with a smaller disparity range ( $D_{max} = 320$ ). It remains inconclusive whether this behavior stems from inherent architectural limitations or a domain gap, as we utilized publicly available pre-trained weights which were likely trained on lower-resolution datasets.

In stark contrast, our S<sup>2</sup>M<sup>2</sup> models demonstrate robust scalability, consistently benefiting from higher-resolution inputs and larger disparity ranges to achieve optimal performance. Furthermore, they exhibit an excellent accuracy-speed trade-off. Even at half resolution, our models, particularly S<sup>2</sup>M<sup>2</sup>-S, provide a highly competitive balance between fast inference and high accuracy, positioning them as an effective solution for various application scenarios.

### 5.3. Analysis of Maximum Disparity Range Impact

This analysis focuses on how the maximum disparity ( $D_{max}$ ) hyperparameter affects models that require it for cost volume construction. Other models that do not use this parameter were excluded from this test, with the exception of our S<sup>2</sup>M<sup>2</sup> model, which is included as a performance baseline. Ideally, for the models under evaluation, increasing the  $D_{max}$  value should improve accuracy, as a larger range covers more ground truth disparities. We investigated this behavior by plotting performance against four  $D_{max}$  values—320, 512, 768, and 960—at both full and half resolutions, as shown in Figure 8 and Figure 9.

However, contrary to this expectation, particularly lightweight models exhibit performance degradation once the  $D_{max}$  value surpasses an optimal threshold. Even a recent model like MoCha [3] showed significant vulnerability to this parameter change. This suggests that an excessively large and sparsely supervised disparity search space can introduce matching ambiguities that some architectures struggle to resolve. It is difficult to definitively conclude whether this is an inherent architectural limitation or a domain gap issue arising from the use of pre-trained weights on datasets with different disparity distributions.

As previously noted, our S<sup>2</sup>M<sup>2</sup> model is unaffected by the  $D_{max}$  parameter. Its consistent performance is therefore shown as a solid line in the figures, serving as a stable reference for comparison.

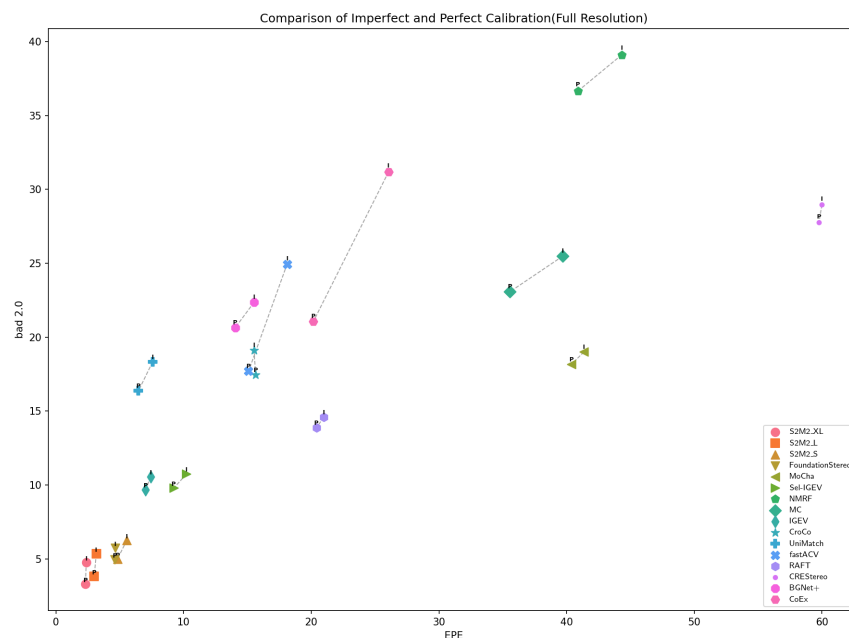

Figure 5. Comparison of model performance under perfect (P) and imperfect (I) calibration settings.

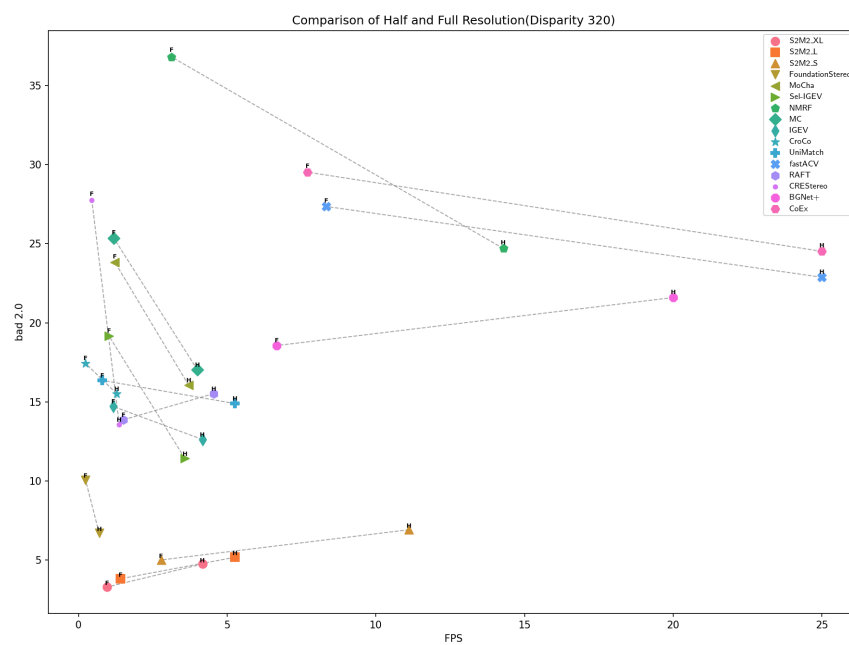

Figure 6. Accuracy vs. inference speed comparison between full (F) and half (H) resolution, with the maximum disparity set to 320. Inference speed was measured with float16 precision using PyTorch's Automatic Mixed Precision (AMP).

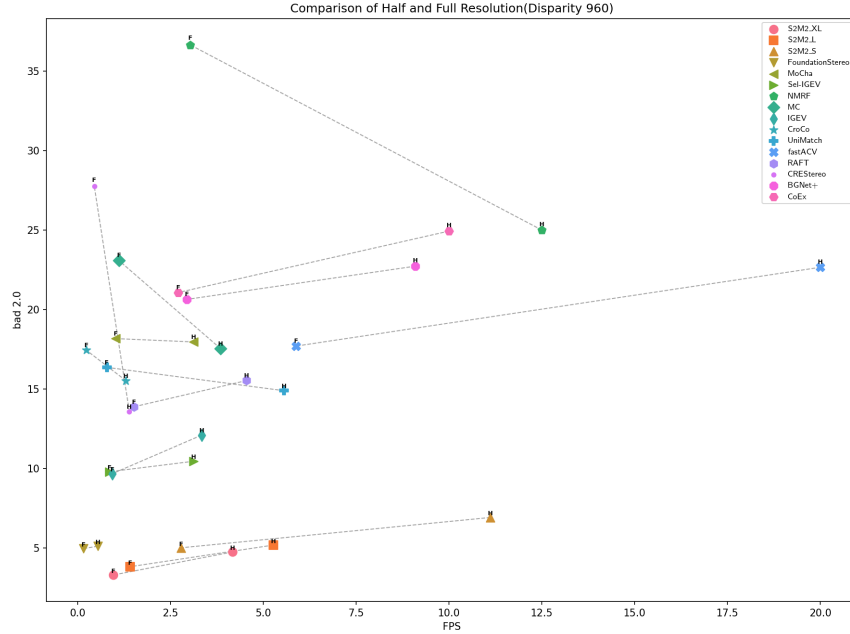

Figure 7. Accuracy vs. inference speed comparison between full (F) and half (H) resolution, with the maximum disparity set to 960. Inference speed was measured with float16 precision using PyTorch’s Automatic Mixed Precision (AMP).

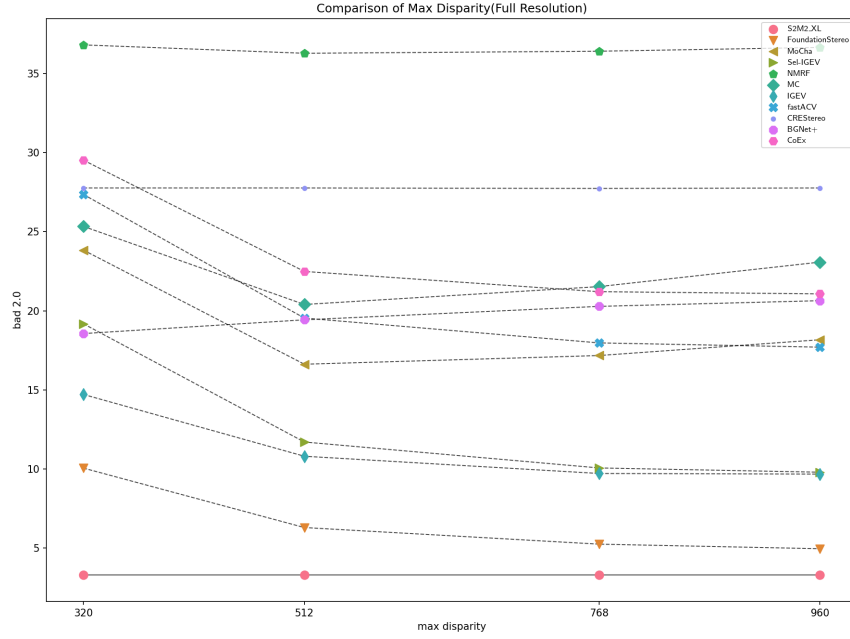

Figure 8. Performance comparison across four maximum disparity ( $D_{max}$ ) settings at full resolution. The solid line indicates our S<sup>2</sup>M<sup>2</sup> model, which is unaffected by this parameter and included for reference.

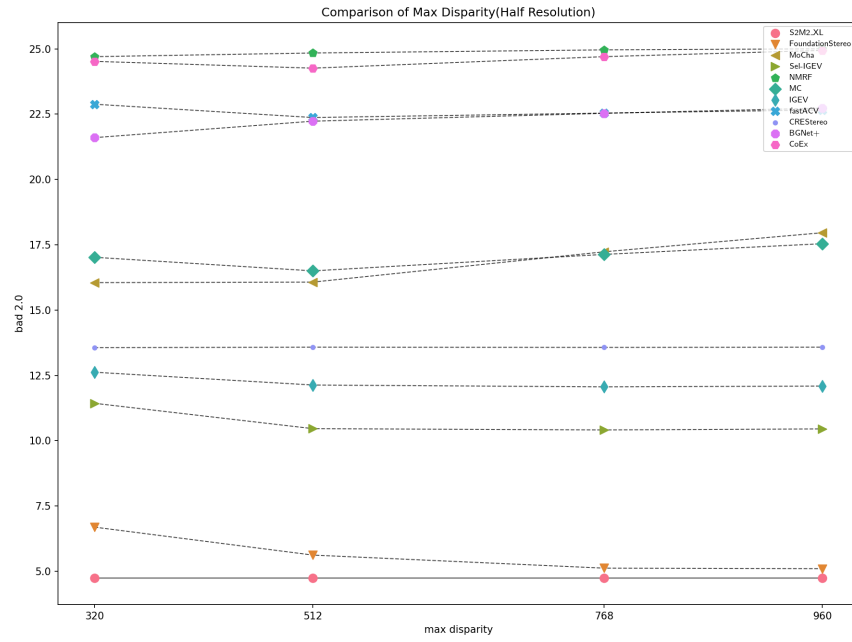

Figure 9. Performance comparison across four maximum disparity ( $D_{max}$ ) settings at half resolution. The solid line indicates our S²M² model, which is unaffected by this parameter and included for reference.

| Model                                       | Non-Occlusion |        |         |         |         |         | All Pixels |         |         |         |         |         |
|---------------------------------------------|---------------|--------|---------|---------|---------|---------|------------|---------|---------|---------|---------|---------|
|                                             | EPE           | RMS    | Bad-0.5 | Bad-1.0 | Bad-2.0 | Bad-4.0 | EPE        | RMS     | Bad-0.5 | Bad-1.0 | Bad-2.0 | Bad-4.0 |
| CoEx [2]                                    | 20.17         | 63.96  | 38.79   | 27.82   | 21.07   | 16.75   | 37.56      | 103.82  | 46.95   | 36.78   | 29.85   | 24.87   |
| BGNet+ [24]                                 | 14.04         | 42.84  | 43.97   | 29.56   | 20.64   | 14.82   | 30.32      | 88      | 50.99   | 37.86   | 29.11   | 22.87   |
| RAFT [10]                                   | 20.41         | 48.13  | 24.43   | 17.73   | 13.88   | 11.33   | 33.09      | 76.53   | 33.33   | 26.45   | 21.84   | 18.32   |
| CREStereo [9]                               | 59.76         | 108.39 | 34.01   | 30.13   | 27.78   | 26.02   | 75.470     | 136.108 | 41.739  | 37.505  | 34.475  | 31.932  |
| fastACV [26]                                | 15.09         | 48.39  | 36.73   | 24.77   | 17.7    | 13.31   | 32.51      | 93.99   | 45.57   | 34.62   | 27.34   | 22.11   |
| UniMatch [27]                               | 6.46          | 17.55  | 55.77   | 31.12   | 16.36   | 10.66   | 13.96      | 37.93   | 61.77   | 40.05   | 25.83   | 18.54   |
| CroCo [22]                                  | 15.65         | 35.66  | 33.83   | 23.72   | 17.44   | 13.48   | 24.99      | 57.23   | 40.7    | 30.96   | 24.32   | 19.57   |
| IGEV [25]                                   | 7.03          | 21.17  | 23.04   | 13.87   | 9.67    | 7.13    | 15.43      | 42.85   | 31.12   | 22.17   | 17.31   | 13.83   |
| MC [5]                                      | 35.57         | 73.77  | 32.48   | 26.72   | 23.08   | 20.57   | 56.07      | 112.67  | 41.13   | 35.48   | 31.47   | 28.3    |
| NMRF [8]                                    | 40.89         | 82.83  | 58.67   | 43.25   | 36.66   | 33.08   | 62.05      | 121.42  | 64.06   | 50.58   | 44.28   | 40.31   |
| Sel-IGEV [20]                               | 9.23          | 25.93  | 22.37   | 14.09   | 9.79    | 7.37    | 18.24      | 48.8    | 30.06   | 21.82   | 16.86   | 13.5    |
| MoCha [3]                                   | 40.38         | 102.65 | 26.9    | 21.63   | 18.17   | 15.73   | 59.75      | 141.2   | 35.34   | 29.91   | 25.94   | 22.82   |
| FoundationStereo [23]                       | 4.61          | 11.28  | 10.96   | 7.23    | 4.95    | 3.49    | 8.26       | 23.05   | 18.43   | 13.98   | 10.73   | 8.09    |
| <b>S<sup>2</sup>M<sup>2</sup>-S (Ours)</b>  | 4.83          | 10.83  | 13.14   | 7.63    | 5       | 3.58    | 9.14       | 26.33   | 20.76   | 14.55   | 10.84   | 8.27    |
| <b>S<sup>2</sup>M<sup>2</sup>-L (Ours)</b>  | 3             | 8.73   | 10.6    | 6.01    | 3.81    | 2.55    | 7.21       | 22.4    | 18.11   | 12.72   | 9.39    | 6.96    |
| <b>S<sup>2</sup>M<sup>2</sup>-XL (Ours)</b> | 2.31          | 7.95   | 9.22    | 5.15    | 3.29    | 2.18    | 6.2        | 20.59   | 16.52   | 11.61   | 8.56    | 6.36    |

Table 3. Stereo matching performance under ideal calibration, full-resolution processing, and a maximum disparity of 960 pixels

| Model                                       | Non-Occlusion |        |         |         |         |         | All Pixels |        |         |         |         |         |
|---------------------------------------------|---------------|--------|---------|---------|---------|---------|------------|--------|---------|---------|---------|---------|
|                                             | EPE           | RMS    | Bad-0.5 | Bad-1.0 | Bad-2.0 | Bad-4.0 | EPE        | RMS    | Bad-0.5 | Bad-1.0 | Bad-2.0 | Bad-4.0 |
| CoEx [2]                                    | 20.48         | 59.68  | 38.87   | 27.93   | 21.21   | 16.93   | 36.72      | 97.04  | 46.97   | 36.8    | 29.88   | 24.92   |
| BGNet+ [24]                                 | 13            | 39.34  | 43.7    | 29.24   | 20.28   | 14.47   | 27.8       | 78.95  | 50.71   | 37.52   | 28.71   | 22.42   |
| RAFT [10]                                   | 20.41         | 48.13  | 24.43   | 17.73   | 13.88   | 11.33   | 33.09      | 76.53  | 33.33   | 26.45   | 21.84   | 18.32   |
| CREStereo [9]                               | 59.73         | 108.33 | 34      | 30.12   | 27.74   | 25.98   | 75.46      | 136.04 | 41.73   | 37.5    | 34.45   | 31.91   |
| fastACV [26]                                | 15.99         | 47.06  | 36.87   | 24.97   | 17.97   | 13.66   | 31.34      | 85.69  | 45.62   | 34.69   | 27.46   | 22.27   |
| UniMatch [27]                               | 6.46          | 17.55  | 55.77   | 31.12   | 16.36   | 10.66   | 13.96      | 37.93  | 61.77   | 40.05   | 25.83   | 18.54   |
| CroCo [22]                                  | 15.65         | 35.66  | 33.83   | 23.72   | 17.44   | 13.48   | 24.99      | 57.23  | 40.7    | 30.96   | 24.32   | 19.57   |
| IGEV [25]                                   | 8.22          | 22.62  | 23.01   | 13.87   | 9.71    | 7.23    | 16.41      | 44.42  | 31.06   | 22.14   | 17.31   | 13.88   |
| MC [5]                                      | 35.75         | 74.82  | 30.92   | 25.11   | 21.53   | 19.1    | 56.07      | 113.4  | 39.58   | 33.82   | 29.83   | 26.73   |
| NMRF [8]                                    | 43.13         | 84.25  | 58.57   | 43.04   | 36.42   | 32.86   | 63.27      | 120.53 | 63.96   | 50.37   | 44.03   | 40.07   |
| Sel-IGEV [20]                               | 11.39         | 29.22  | 22.28   | 14.12   | 10.06   | 7.72    | 20.36      | 51.78  | 29.98   | 21.84   | 17.06   | 13.8    |
| MoCha [3]                                   | 35.94         | 93.17  | 25.96   | 20.65   | 17.17   | 14.74   | 52.84      | 128.02 | 34.44   | 28.95   | 24.91   | 21.74   |
| FoundationStereo [23]                       | 4.61          | 11     | 11.35   | 7.6     | 5.24    | 3.67    | 8.38       | 23.43  | 18.72   | 14.28   | 10.98   | 8.27    |
| <b>S<sup>2</sup>M<sup>2</sup>-S (Ours)</b>  | 4.83          | 10.83  | 13.14   | 7.63    | 5       | 3.58    | 9.14       | 26.33  | 20.76   | 14.55   | 10.84   | 8.27    |
| <b>S<sup>2</sup>M<sup>2</sup>-L (Ours)</b>  | 3             | 8.73   | 10.6    | 6.01    | 3.81    | 2.55    | 7.21       | 22.4   | 18.11   | 12.72   | 9.39    | 6.96    |
| <b>S<sup>2</sup>M<sup>2</sup>-XL (Ours)</b> | 2.31          | 7.95   | 9.22    | 5.15    | 3.29    | 2.18    | 6.2        | 20.59  | 16.52   | 11.61   | 8.56    | 6.36    |

Table 4. Stereo matching performance under ideal calibration, full-resolution processing, and a maximum disparity of 768 pixels

| Model                                       | Non-Occlusion |        |         |         |         |         | All Pixels |        |         |         |         |         |
|---------------------------------------------|---------------|--------|---------|---------|---------|---------|------------|--------|---------|---------|---------|---------|
|                                             | EPE           | RMS    | Bad-0.5 | Bad-1.0 | Bad-2.0 | Bad-4.0 | EPE        | RMS    | Bad-0.5 | Bad-1.0 | Bad-2.0 | Bad-4.0 |
| CoEx [2]                                    | 26.71         | 66.6   | 39.62   | 28.97   | 22.49   | 18.38   | 41.96      | 97.98  | 47.51   | 37.56   | 30.83   | 26.01   |
| BGNet+ [24]                                 | 12.34         | 36.5   | 42.96   | 28.37   | 19.43   | 13.71   | 26.96      | 73.15  | 50.04   | 36.72   | 27.87   | 21.61   |
| RAFT [10]                                   | 20.41         | 48.13  | 24.43   | 17.73   | 13.88   | 11.33   | 33.08      | 76.53  | 33.31   | 26.43   | 21.84   | 18.31   |
| CREStereo [9]                               | 59.76         | 108.39 | 34.01   | 30.13   | 27.78   | 26.02   | 75.47      | 136.11 | 41.74   | 37.51   | 34.48   | 31.93   |
| fastACV [26]                                | 23.11         | 57.32  | 37.73   | 26.2    | 19.54   | 15.47   | 37.7       | 88.49  | 46.26   | 35.62   | 28.66   | 23.69   |
| UniMatch [27]                               | 6.46          | 17.55  | 55.77   | 31.12   | 16.36   | 10.66   | 13.96      | 37.93  | 61.77   | 40.05   | 25.83   | 18.54   |
| CroCo [22]                                  | 15.65         | 35.66  | 33.83   | 23.72   | 17.44   | 13.48   | 24.99      | 57.23  | 40.7    | 30.96   | 24.32   | 19.57   |
| IGEV [25]                                   | 11.39         | 27.51  | 23.7    | 14.85   | 10.8    | 8.41    | 20.64      | 51.54  | 31.62   | 22.98   | 18.31   | 15.02   |
| MC [5]                                      | 39.17         | 82.69  | 29.56   | 23.84   | 20.4    | 18.16   | 59.11      | 119.61 | 38.22   | 32.51   | 28.63   | 25.72   |
| NMRF [8]                                    | 51.34         | 95.78  | 58.42   | 42.84   | 36.29   | 32.85   | 69.79      | 127.5  | 63.8    | 50.12   | 43.78   | 39.87   |
| Sel-IGEV [20]                               | 17.14         | 41.15  | 22.61   | 15.27   | 11.7    | 9.6     | 27.71      | 65.13  | 30.26   | 22.79   | 18.47   | 15.53   |
| MoCha [3]                                   | 23.19         | 58.08  | 25.4    | 20.1    | 16.62   | 14.18   | 34.84      | 83.37  | 33.76   | 28.23   | 24.12   | 20.89   |
| FoundationStereo [23]                       | 4.7           | 12.26  | 13.27   | 9.35    | 6.29    | 4.17    | 9.71       | 26.57  | 20.32   | 15.83   | 12.06   | 9.01    |
| <b>S<sup>2</sup>M<sup>2</sup>-S (Ours)</b>  | 4.83          | 10.83  | 13.14   | 7.63    | 5       | 3.58    | 9.14       | 26.33  | 20.76   | 14.55   | 10.84   | 8.27    |
| <b>S<sup>2</sup>M<sup>2</sup>-L (Ours)</b>  | 3             | 8.73   | 10.6    | 6.01    | 3.81    | 2.55    | 7.21       | 22.4   | 18.11   | 12.72   | 9.39    | 6.96    |
| <b>S<sup>2</sup>M<sup>2</sup>-XL (Ours)</b> | 2.31          | 7.95   | 9.22    | 5.15    | 3.29    | 2.18    | 6.2        | 20.59  | 16.52   | 11.61   | 8.56    | 6.36    |

Table 5. Stereo matching performance under ideal calibration, full-resolution processing, and a maximum disparity of 512 pixels

| Model                                       | Non-Occlusion |        |         |         |         |         | All Pixels |        |         |         |         |         |
|---------------------------------------------|---------------|--------|---------|---------|---------|---------|------------|--------|---------|---------|---------|---------|
|                                             | EPE           | RMS    | Bad-0.5 | Bad-1.0 | Bad-2.0 | Bad-4.0 | EPE        | RMS    | Bad-0.5 | Bad-1.0 | Bad-2.0 | Bad-4.0 |
| CoEx [2]                                    | 44.89         | 91.33  | 44.61   | 35.23   | 29.53   | 25.84   | 60.47      | 119.26 | 51.49   | 42.6    | 36.58   | 32.21   |
| BGNet+ [24]                                 | 17.37         | 45.41  | 41.92   | 27.25   | 18.56   | 13.46   | 32.39      | 80.95  | 49.14   | 35.71   | 27.02   | 21.21   |
| RAFT [10]                                   | 20.41         | 48.14  | 24.41   | 17.71   | 13.87   | 11.33   | 33.08      | 76.53  | 33.31   | 26.43   | 21.84   | 18.31   |
| CREStereo [9]                               | 59.72         | 108.43 | 33.99   | 30.12   | 27.77   | 26.03   | 75.5       | 136.23 | 41.71   | 37.49   | 34.47   | 31.94   |
| fastACV [26]                                | 41.78         | 85.57  | 42.94   | 33.04   | 27.36   | 23.78   | 57.07      | 113.14 | 50.41   | 41.13   | 35.06   | 30.62   |
| UniMatch [27]                               | 6.46          | 17.55  | 55.77   | 31.12   | 16.36   | 10.66   | 13.96      | 37.93  | 61.77   | 40.05   | 25.83   | 18.54   |
| CroCo [22]                                  | 15.65         | 35.66  | 33.83   | 23.72   | 17.44   | 13.48   | 24.99      | 57.23  | 40.7    | 30.96   | 24.32   | 19.57   |
| IGEV [25]                                   | 17.63         | 39.4   | 27.24   | 18.9    | 14.71   | 12.24   | 28.07      | 63.98  | 34.6    | 26.48   | 21.81   | 18.56   |
| MC [5]                                      | 57.99         | 109.5  | 33.44   | 28.44   | 25.34   | 23.26   | 76.54      | 141.84 | 41.28   | 36.16   | 32.57   | 29.82   |
| NMRF [8]                                    | 64.57         | 112.58 | 58.31   | 43.03   | 36.82   | 33.67   | 80.97      | 140.38 | 63.66   | 50.18   | 44.08   | 40.39   |
| Sel-IGEV [20]                               | 31.46         | 64.73  | 27.94   | 22.14   | 19.18   | 17.35   | 44.41      | 90.7   | 34.94   | 28.92   | 25.3    | 22.75   |
| MoCha [3]                                   | 39.56         | 81.83  | 31.36   | 26.81   | 23.84   | 21.75   | 53.55      | 108    | 38.59   | 33.78   | 30.23   | 27.48   |
| FoundationStereo [23]                       | 7.88          | 17.41  | 22.04   | 16.71   | 10.05   | 5.77    | 13.22      | 33.06  | 28.27   | 22.64   | 15.87   | 10.88   |
| <b>S<sup>2</sup>M<sup>2</sup>-S (Ours)</b>  | 4.83          | 10.83  | 13.14   | 7.63    | 5       | 3.58    | 9.14       | 26.33  | 20.76   | 14.55   | 10.84   | 8.27    |
| <b>S<sup>2</sup>M<sup>2</sup>-L (Ours)</b>  | 3             | 8.73   | 10.6    | 6.01    | 3.81    | 2.55    | 7.21       | 22.4   | 18.11   | 12.72   | 9.39    | 6.96    |
| <b>S<sup>2</sup>M<sup>2</sup>-XL (Ours)</b> | 2.31          | 7.95   | 9.22    | 5.15    | 3.29    | 2.18    | 6.2        | 20.59  | 16.52   | 11.61   | 8.56    | 6.36    |

Table 6. Stereo matching performance under ideal calibration, full-resolution processing, and a maximum disparity of 320 pixels

| Model                                       | Non-Occlusion |        |         |         |         |         | All Pixels |        |         |         |         |         |
|---------------------------------------------|---------------|--------|---------|---------|---------|---------|------------|--------|---------|---------|---------|---------|
|                                             | EPE           | RMS    | Bad-0.5 | Bad-1.0 | Bad-2.0 | Bad-4.0 | EPE        | RMS    | Bad-0.5 | Bad-1.0 | Bad-2.0 | Bad-4.0 |
| CoEx [2]                                    | 26.05         | 77.03  | 57.65   | 42.68   | 31.18   | 23.55   | 42.98      | 113.25 | 63.38   | 49.87   | 38.91   | 31.07   |
| BGNet+ [24]                                 | 15.52         | 46.03  | 46.27   | 31.93   | 22.36   | 16.28   | 31.66      | 90.03  | 53.01   | 39.96   | 30.69   | 24.25   |
| RAFT [10]                                   | 20.98         | 49.17  | 26.08   | 18.7    | 14.58   | 11.85   | 33.98      | 78.01  | 34.76   | 27.29   | 22.44   | 18.78   |
| CREStereo [9]                               | 60            | 108.29 | 35.98   | 31.69   | 28.96   | 26.96   | 75.58      | 136.01 | 43.45   | 38.85   | 35.5    | 32.75   |
| fastACV [26]                                | 18.11         | 56.18  | 51.1    | 36.02   | 24.95   | 17.99   | 35.3       | 98.62  | 57.94   | 44.37   | 33.77   | 26.34   |
| UniMatch [27]                               | 7.57          | 20.17  | 59.7    | 35.13   | 18.32   | 11.67   | 15.28      | 40.57  | 65.18   | 43.55   | 27.6    | 19.5    |
| CroCo [22]                                  | 15.51         | 35.54  | 38.2    | 26.51   | 19.11   | 14.43   | 24.95      | 57.23  | 44.64   | 33.47   | 25.82   | 20.45   |
| IGEV [25]                                   | 7.42          | 21.82  | 24.78   | 15.14   | 10.56   | 7.9     | 15.68      | 42.94  | 32.61   | 23.28   | 18.11   | 14.49   |
| MC [5]                                      | 39.69         | 80.89  | 35.35   | 29.24   | 25.48   | 22.86   | 59.86      | 118.23 | 43.57   | 37.63   | 33.53   | 30.29   |
| NMRF [8]                                    | 44.32         | 89.59  | 62.92   | 47.43   | 39.11   | 34.75   | 64.83      | 125.78 | 67.86   | 54.28   | 46.45   | 41.81   |
| Sel-IGEV [20]                               | 10.22         | 28.25  | 24.29   | 15.57   | 10.73   | 8.19    | 19.23      | 50.69  | 31.69   | 23.11   | 17.76   | 14.3    |
| MoCha [3]                                   | 41.36         | 103.89 | 28.25   | 22.66   | 19      | 16.41   | 60.75      | 142.22 | 36.52   | 30.84   | 26.72   | 23.5    |
| FoundationStereo [23]                       | 4.66          | 11.25  | 12.44   | 8.32    | 5.74    | 3.96    | 8.13       | 22.34  | 19.85   | 15.07   | 11.52   | 8.62    |
| <b>S<sup>2</sup>M<sup>2</sup>-S (Ours)</b>  | 5.55          | 11.68  | 16.64   | 9.72    | 6.25    | 4.09    | 9.88       | 27.12  | 24.04   | 16.58   | 12.08   | 8.85    |
| <b>S<sup>2</sup>M<sup>2</sup>-L (Ours)</b>  | 3.16          | 9.21   | 14.36   | 8.42    | 5.33    | 3.39    | 7.38       | 22.6   | 21.69   | 15.07   | 10.95   | 7.9     |
| <b>S<sup>2</sup>M<sup>2</sup>-XL (Ours)</b> | 2.38          | 8.04   | 12.93   | 7.45    | 4.77    | 3.07    | 6.15       | 20.49  | 20.11   | 13.89   | 10.16   | 7.4     |

Table 7. Stereo matching performance under non-ideal calibration, full-resolution processing, and a maximum disparity of 960 pixels

| Model                                       | Non-Occlusion |        |         |         |         |         | All Pixels |        |         |         |         |         |
|---------------------------------------------|---------------|--------|---------|---------|---------|---------|------------|--------|---------|---------|---------|---------|
|                                             | EPE           | RMS    | Bad-0.5 | Bad-1.0 | Bad-2.0 | Bad-4.0 | EPE        | RMS    | Bad-0.5 | Bad-1.0 | Bad-2.0 | Bad-4.0 |
| CoEx [2]                                    | 47.03         | 94.34  | 60.24   | 46.73   | 36.65   | 30.2    | 62.56      | 121.81 | 65.36   | 52.97   | 43.17   | 36.33   |
| BGNet+ [24]                                 | 18.64         | 48.16  | 44.26   | 29.66   | 20.26   | 14.83   | 33.66      | 82.75  | 51.2    | 37.85   | 28.58   | 22.5    |
| RAFT [10]                                   | 20.96         | 49.12  | 26.09   | 18.71   | 14.57   | 11.84   | 33.96      | 77.97  | 34.76   | 27.3    | 22.43   | 18.76   |
| CREStereo [9]                               | 60            | 108.3  | 35.96   | 31.66   | 28.95   | 26.94   | 75.6       | 136.02 | 43.44   | 38.83   | 35.48   | 32.73   |
| fastACV [26]                                | 42.51         | 86.37  | 54.44   | 41.15   | 31.9    | 26.23   | 57.77      | 113.74 | 60.51   | 48.36   | 39.23   | 32.96   |
| UniMatch [27]                               | 7.57          | 20.17  | 59.7    | 35.13   | 18.32   | 11.67   | 15.28      | 40.57  | 65.18   | 43.55   | 27.6    | 19.5    |
| CroCo [22]                                  | 15.51         | 35.54  | 38.2    | 26.51   | 19.11   | 14.43   | 24.95      | 57.23  | 44.64   | 33.47   | 25.82   | 20.45   |
| IGEV [25]                                   | 18.16         | 40.42  | 28.7    | 20.22   | 15.74   | 13.09   | 28.36      | 64.06  | 35.89   | 27.66   | 22.71   | 19.28   |
| MC [5]                                      | 59.01         | 110.92 | 34.99   | 29.47   | 26.22   | 24.06   | 77.65      | 143.2  | 42.64   | 37.1    | 33.4    | 30.59   |
| NMRF [8]                                    | 64.98         | 112.83 | 62.27   | 46.73   | 38.63   | 34.67   | 81.26      | 140.41 | 67.22   | 53.49   | 45.75   | 41.34   |
| Sel-IGEV [20]                               | 31.94         | 65.66  | 29.01   | 23      | 19.82   | 17.87   | 44.79      | 91.26  | 35.86   | 29.66   | 25.86   | 23.19   |
| MoCha [3]                                   | 39.63         | 81.88  | 32.28   | 27.52   | 24.36   | 22.08   | 53.72      | 108.27 | 39.41   | 34.39   | 30.7    | 27.79   |
| FoundationStereo [23]                       | 8.03          | 17.38  | 23.25   | 17.87   | 12.55   | 8.09    | 13.27      | 32.67  | 29.39   | 23.7    | 18.01   | 12.97   |
| <b>S<sup>2</sup>M<sup>2</sup>-S (Ours)</b>  | 5.55          | 11.68  | 16.64   | 9.72    | 6.25    | 4.09    | 9.88       | 27.12  | 24.04   | 16.58   | 12.08   | 8.85    |
| <b>S<sup>2</sup>M<sup>2</sup>-L (Ours)</b>  | 3.16          | 9.21   | 14.36   | 8.42    | 5.33    | 3.39    | 7.38       | 22.6   | 21.69   | 15.07   | 10.95   | 7.9     |
| <b>S<sup>2</sup>M<sup>2</sup>-XL (Ours)</b> | 2.38          | 8.04   | 12.93   | 7.45    | 4.77    | 3.07    | 6.15       | 20.49  | 20.11   | 13.89   | 10.16   | 7.4     |

Table 8. Stereo matching performance under non-ideal calibration, full-resolution processing, and a maximum disparity of 320 pixels

| Model                                       | Non-Occlusion |        |         |         |         |         | All Pixels |        |         |         |         |         |
|---------------------------------------------|---------------|--------|---------|---------|---------|---------|------------|--------|---------|---------|---------|---------|
|                                             | EPE           | RMS    | Bad-0.5 | Bad-1.0 | Bad-2.0 | Bad-4.0 | EPE        | RMS    | Bad-0.5 | Bad-1.0 | Bad-2.0 | Bad-4.0 |
| CoEx [2]                                    | 29.26         | 106.76 | 53.33   | 36.77   | 24.94   | 17.69   | 44.19      | 141.71 | 59.3    | 44.45   | 33.13   | 25.37   |
| BGNet+ [24]                                 | 11.38         | 37.92  | 56.55   | 36.97   | 22.73   | 14.54   | 27.89      | 82.32  | 61.89   | 44.27   | 30.77   | 22.11   |
| RAFT [10]                                   | 11.19         | 28.53  | 35.6    | 22.94   | 15.52   | 11.2    | 20.77      | 51.47  | 43.24   | 31.23   | 23.46   | 18.24   |
| CREStereo [9]                               | 18.7          | 43.39  | 27.68   | 18.69   | 13.58   | 10.53   | 29.26      | 67.07  | 36.31   | 27.48   | 21.69   | 17.62   |
| fastACV [26]                                | 18.03         | 65.25  | 53.29   | 35.45   | 22.66   | 15.06   | 32.96      | 105.21 | 59.52   | 43.75   | 31.71   | 23.52   |
| UniMatch [27]                               | 5.67          | 16.71  | 48.13   | 26.16   | 14.89   | 9.56    | 13.06      | 36.21  | 54.44   | 34.55   | 23.3    | 16.86   |
| CroCo [22]                                  | 8.51          | 21.89  | 39.14   | 24.87   | 15.52   | 10.22   | 15.62      | 40.69  | 45.14   | 31.61   | 22.12   | 16      |
| IGEV [25]                                   | 7.76          | 20.32  | 33.76   | 19.73   | 12.09   | 8.01    | 14.99      | 40.17  | 40.24   | 27.02   | 19.15   | 14.24   |
| MC [5]                                      | 17.51         | 42.45  | 34.63   | 24.21   | 17.54   | 13.32   | 32.2       | 74.02  | 42.58   | 32.75   | 25.85   | 20.86   |
| NMRF [8]                                    | 24.45         | 65.77  | 57.77   | 38.65   | 25      | 18.21   | 41.16      | 99.98  | 63.28   | 46.42   | 33.75   | 26.54   |
| Sel-IGEV [20]                               | 7.09          | 20.45  | 29.46   | 17.31   | 10.45   | 6.8     | 14.43      | 40.69  | 36.31   | 24.65   | 17.38   | 12.78   |
| MoCha [3]                                   | 26.8          | 90.02  | 32.89   | 23.77   | 17.96   | 14.26   | 42.88      | 125.07 | 40.35   | 31.51   | 25.38   | 20.97   |
| FoundationStereo [23]                       | 2.65          | 11.57  | 14.98   | 8.68    | 5.1     | 3.06    | 7.13       | 23.51  | 22.13   | 15.36   | 10.76   | 7.56    |
| <b>S<sup>2</sup>M<sup>2</sup>-S (Ours)</b>  | 2.77          | 9.73   | 23.84   | 12.73   | 6.91    | 4.05    | 8          | 26.11  | 30.79   | 19.79   | 13.27   | 9.24    |
| <b>S<sup>2</sup>M<sup>2</sup>-L (Ours)</b>  | 2.57          | 8.52   | 18.78   | 9.42    | 5.17    | 3.14    | 6.63       | 22.03  | 25.8    | 16.2    | 10.96   | 7.73    |
| <b>S<sup>2</sup>M<sup>2</sup>-XL (Ours)</b> | 2.83          | 8.91   | 17.09   | 8.48    | 4.74    | 2.91    | 6.53       | 21.71  | 23.96   | 15.04   | 10.25   | 7.23    |

Table 9. Stereo matching performance under non-ideal calibration, half-resolution processing, and a maximum disparity of 960 pixels

| Model                                       | Non-Occlusion |       |         |         |         |         | All Pixels |       |         |         |         |         |
|---------------------------------------------|---------------|-------|---------|---------|---------|---------|------------|-------|---------|---------|---------|---------|
|                                             | EPE           | RMS   | Bad-0.5 | Bad-1.0 | Bad-2.0 | Bad-4.0 | EPE        | RMS   | Bad-0.5 | Bad-1.0 | Bad-2.0 | Bad-4.0 |
| CoEx [2]                                    | 20.06         | 53.35 | 53.09   | 36.42   | 24.52   | 17.26   | 31.66      | 79.32 | 59.02   | 44.03   | 32.58   | 24.73   |
| BGNet+ [24]                                 | 8.44          | 24.21 | 55.89   | 36      | 21.6    | 13.48   | 18.83      | 51.03 | 61.26   | 43.32   | 29.6    | 20.88   |
| RAFT [10]                                   | 11.19         | 28.53 | 35.6    | 22.94   | 15.52   | 11.2    | 20.77      | 51.47 | 43.24   | 31.23   | 23.46   | 18.24   |
| CREStereo [9]                               | 18.77         | 43.8  | 27.66   | 18.66   | 13.56   | 10.51   | 29.33      | 67.32 | 36.31   | 27.46   | 21.69   | 17.61   |
| fastACV [26]                                | 17.64         | 45.86 | 52.87   | 35.24   | 22.88   | 15.62   | 28.23      | 70.78 | 59.08   | 43.46   | 31.74   | 23.84   |
| UniMatch [27]                               | 5.67          | 16.71 | 48.13   | 26.16   | 14.89   | 9.56    | 13.06      | 36.21 | 54.44   | 34.55   | 23.3    | 16.86   |
| CroCo [22]                                  | 8.51          | 21.89 | 39.14   | 24.87   | 15.52   | 10.22   | 15.62      | 40.69 | 45.14   | 31.61   | 22.12   | 16      |
| IGEV [25]                                   | 10.83         | 24.02 | 33.89   | 20.11   | 12.62   | 8.55    | 17.91      | 43.9  | 40.37   | 27.36   | 19.64   | 14.76   |
| MC [5]                                      | 22.8          | 51.51 | 33.67   | 23.44   | 17.06   | 13.11   | 36.82      | 81.6  | 41.46   | 31.72   | 24.99   | 20.21   |
| NMRF [8]                                    | 27.28         | 62.17 | 57.64   | 38.34   | 24.7    | 17.99   | 41.94      | 90.94 | 63.14   | 46.08   | 33.4    | 26.23   |
| Sel-IGEV [20]                               | 11.89         | 28.12 | 29.75   | 18.04   | 11.43   | 7.98    | 19.99      | 49.03 | 36.59   | 25.3    | 18.29   | 13.92   |
| MoCha [3]                                   | 15.2          | 41.72 | 30.74   | 21.61   | 16.05   | 12.49   | 24.79      | 64.05 | 38.24   | 29.3    | 23.29   | 18.89   |
| FoundationStereo [23]                       | 3.92          | 11.24 | 16.7    | 10.52   | 6.7     | 4.28    | 8.33       | 24.52 | 23.45   | 16.81   | 12.15   | 8.74    |
| <b>S<sup>2</sup>M<sup>2</sup>-S (Ours)</b>  | 2.77          | 9.73  | 23.84   | 12.73   | 6.91    | 4.05    | 8          | 26.11 | 30.79   | 19.79   | 13.27   | 9.24    |
| <b>S<sup>2</sup>M<sup>2</sup>-L (Ours)</b>  | 2.57          | 8.52  | 18.78   | 9.42    | 5.17    | 3.14    | 6.63       | 22.03 | 25.8    | 16.2    | 10.96   | 7.73    |
| <b>S<sup>2</sup>M<sup>2</sup>-XL (Ours)</b> | 2.83          | 8.91  | 17.09   | 8.48    | 4.74    | 2.91    | 6.53       | 21.71 | 23.96   | 15.04   | 10.25   | 7.23    |

Table 10. Stereo matching performance under non-ideal calibration, half-resolution processing, and a maximum disparity of 320 pixels

# 6. Real-world Benchmarks

Our model’s state-of-the-art performance on real-world data is demonstrated by its rankings on the competitive ETH3D [15] and Middlebury v3 [14] benchmarks. As of July 2025, our model ranks first on both leaderboards. Snapshots of the official leaderboards are shown in Figure 10 and Figure 11.

ETH3D

HomeStereoSLAMAboutSubmit

Low-res two-view benchmark

This table lists the benchmark results for the low-res two-view scenario. This benchmark evaluates the [Middlebury stereo](#) metrics (for all metrics, smaller is better):

- **bad 0.5, 1.0, 2.0, 4.0 [%]**: Fraction of pixels with errors larger than the given number of disparities.
- **Average error [px]**: The per-pixel average disparity error.
- **Root mean square error [px]**: The per-pixel root mean square disparity error.
- **50%, 90%, 95%, 99% error quantile [px]**: The highest disparity error within the given percentage of best pixels (for 50%, this is the median error).
- **Time [s]**: The runtime of the method.

The mask determines whether the metric is evaluated for all pixels with ground truth, or only for pixels which are visible in both images (non-occluded). The coverage selector allows to limit the table to results for all pixels (dense), or a given minimum fraction of pixels.

Methods with suffix\_ROB may participate in the [Robust Vision Challenge](#).

Click one or more dataset result cells or column headers to show visualizations. Most visualizations are only available for [training datasets](#). The visualizations may not work with mobile browsers.

Coverage: denseSet: TestMetric: bad 1.0 [%]Mask: non-occluded

Download this table as CSV

| Method           | Info | all  | lakes. 1l | lakes. 1s | sand box 1l | sand box 1s | stora. room 1l | stora. room 1s | stora. room 2l | stora. room 2s | stora. room 2 1l | stora. room 2 1s | stora. room 2 2l | stora. room 2 2s | stora. room 3l | stora. room 3s | tunnel 1l | tunnel 1s | tunnel 2l |
|------------------|------|------|-----------|-----------|-------------|-------------|----------------|----------------|----------------|----------------|------------------|------------------|------------------|------------------|----------------|----------------|-----------|-----------|-----------|
| S2M2_XL          |      | 0.22 | 0.33      | 1.17      | 0.07        | 0.11        | 0.11           | 0.00           | 0.60           | 0.25           | 0.12             | 0.73             | 0.07             | 0.17             | 0.39           | 0.20           | 0.00      | 0.01      | 0.00      |
| FoundationStereo |      | 0.26 | 0.29      | 1.25      | 0.24        | 0.10        | 0.41           | 0.07           | 0.57           | 0.80           | 0.24             | 0.03             | 0.09             | 0.37             | 0.46           | 0.12           | 0.03      | 0.03      | 0.00      |
| LGtest1          |      | 0.42 | 0.33      | 1.42      | 0.13        | 0.16        | 0.98           | 0.01           | 2.30           | 0.96           | 0.21             | 0.07             | 0.08             | 0.10             | 1.10           | 0.31           | 0.01      | 0.09      | 0.00      |
| 3.25w_new        |      | 0.45 | 0.25      | 1.29      | 0.02        | 0.08        | 1.25           | 0.01           | 3.39           | 0.91           | 0.33             | 0.16             | 0.07             | 0.42             | 0.57           | 0.25           | 0.00      | 0.00      | 0.00      |
| 3.25w            |      | 0.45 | 0.25      | 1.29      | 0.02        | 0.08        | 1.25           | 0.01           | 3.39           | 0.91           | 0.33             | 0.16             | 0.06             | 0.42             | 0.57           | 0.25           | 0.00      | 0.00      | 0.00      |
| MLG-Stereo_test3 |      | 0.45 | 0.31      | 1.35      | 0.06        | 0.17        | 1.30           | 0.01           | 3.52           | 0.77           | 0.15             | 0.07             | 0.06             | 0.07             | 0.74           | 0.22           | 0.02      | 0.06      | 0.00      |
| S2M2             |      | 0.46 | 0.39      | 1.17      | 0.37        | 0.17        | 1.14           | 0.01           | 1.46           | 1.83           | 0.19             | 0.87             | 0.13             | 0.19             | 0.57           | 0.43           | 0.01      | 0.01      | 0.00      |
| MonSter          |      | 0.46 | 0.23      | 1.44      | 0.05        | 0.77        | 1.17           | 0.01           | 3.17           | 0.72           | 0.28             | 0.18             | 0.07             | 0.04             | 0.83           | 0.17           | 0.00      | 0.00      | 0.00      |
| asd              |      | 0.49 | 0.16      | 1.57      | 0.04        | 0.72        | 1.24           | 0.05           | 2.80           | 0.84           | 0.45             | 0.50             | 0.06             | 0.56             | 0.58           | 0.24           | 0.00      | 0.00      | 0.00      |
| 4.5_new          |      | 0.49 | 0.17      | 1.73      | 0.06        | 0.30        | 1.23           | 0.07           | 3.11           | 0.87           | 0.45             | 0.66             | 0.05             | 0.19             | 0.67           | 0.26           | 0.00      | 0.00      | 0.00      |
| 4.5w-stereo      |      | 0.49 | 0.17      | 1.73      | 0.06        | 0.30        | 1.23           | 0.07           | 3.11           | 0.87           | 0.45             | 0.66             | 0.05             | 0.19             | 0.67           | 0.26           | 0.00      | 0.00      | 0.00      |
| IGEV             |      | 0.50 | 0.22      | 1.52      | 0.08        | 1.85        | 1.34           | 0.37           | 2.03           | 0.93           | 0.29             | 0.08             | 0.07             | 0.09             | 0.90           | 0.22           | 0.02      | 0.04      | 0.00      |

Figure 10. Snapshot of the official ETH3D low-resolution stereo benchmark leaderboard, taken in July 2025. Our model holds the top-ranking position, outperforming prior state-of-the-art methods.

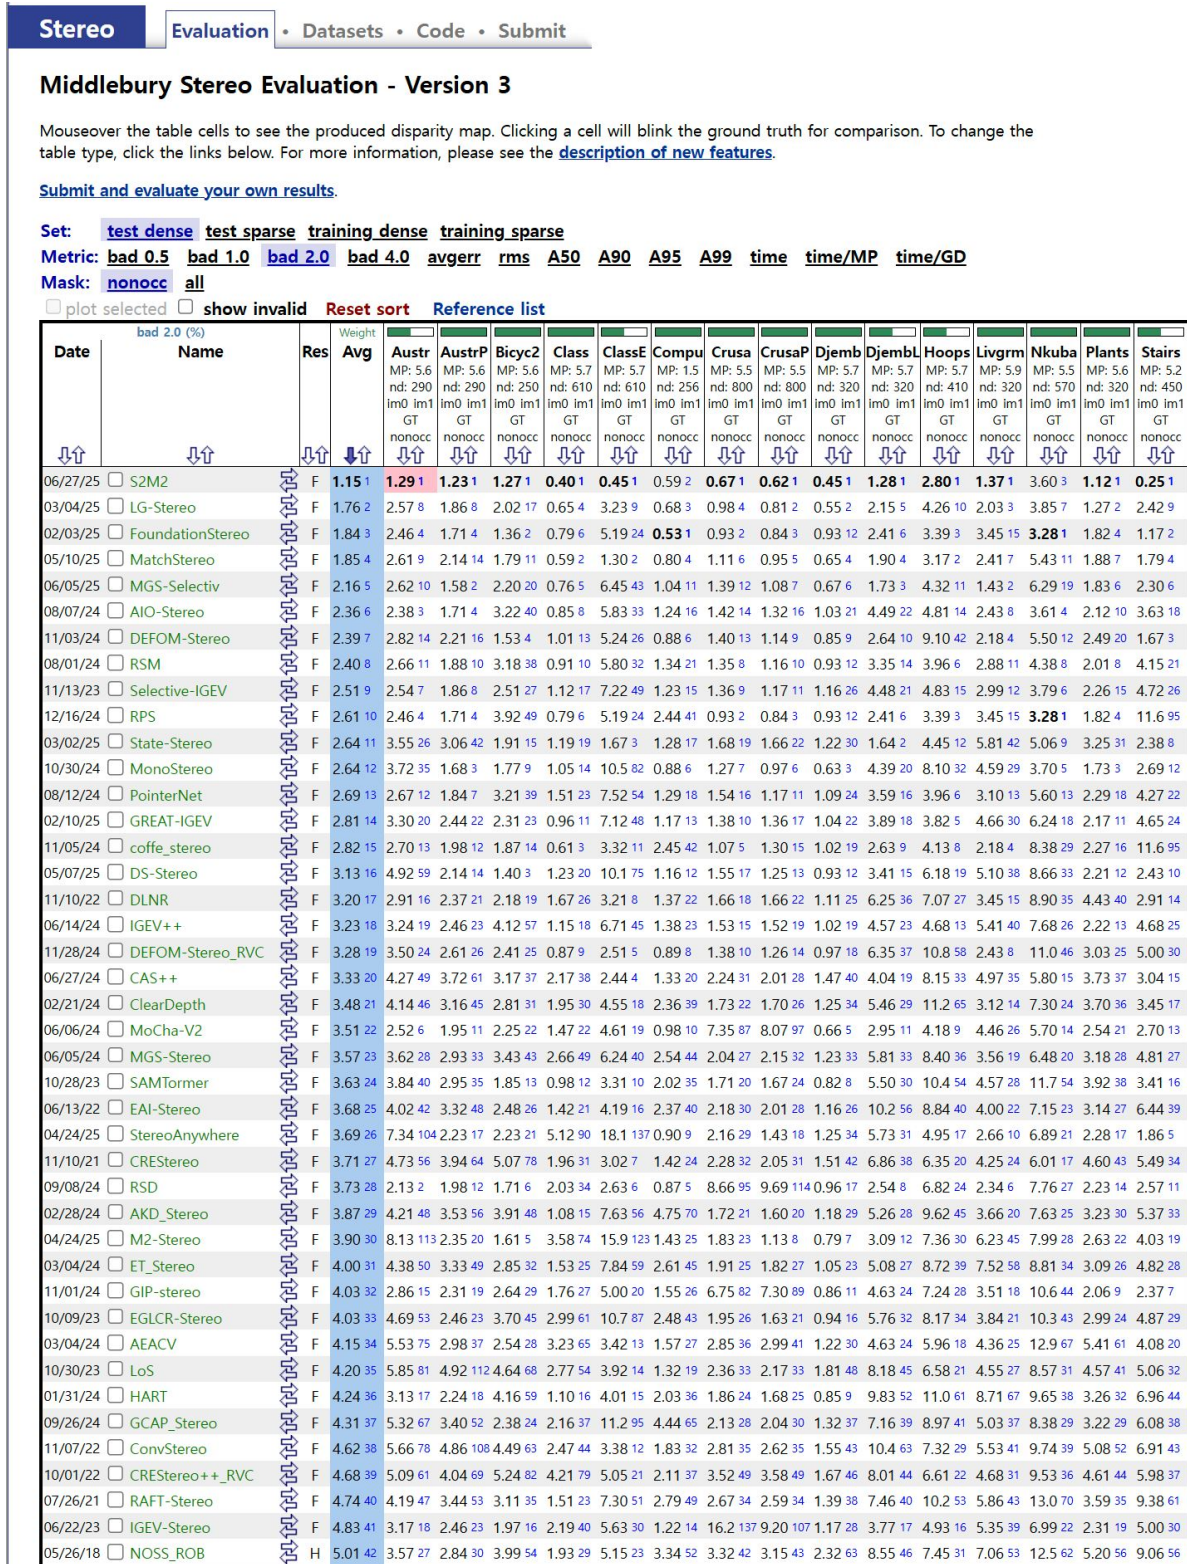

Figure 11. Snapshot of the official Middlebury v3 benchmark leaderboard, taken in July 2025. Our model is ranked first, demonstrating its robust and accurate performance.

## References

- [1] Blenderkit. <https://www.blenderkit.com/> [Accessed: (2024)].
- [2] Antyanta Bangunharcana, Jae Won Cho, Seokju Lee, In So Kweon, Kyung-Soo Kim, and Soohyun Kim. Correlate-and-excite: Real-time stereo matching via guided cost volume excitation. In *IEEE/RSJ International Conference on Intelligent Robots and Systems (IROS)*, pages 3542–3548. IEEE, 2021.
- [3] Ziyang Chen, Wei Long, He Yao, Yongjun Zhang, Bingshu Wang, Yongbin Qin, and Jia Wu. Mocha-stereo: Motif channel attention network for stereo matching. In *Proceedings of the IEEE/CVF Conference on Computer Vision and Pattern Recognition*, pages 27768–27777, 2024.
- [4] Matt Deitke, Dustin Schwenk, Jordi Salvador, Luca Weihs, Oscar Michel, Eli VanderBilt, Ludwig Schmidt, Kiana Ehsani, Aniruddha Kembhavi, and Ali Farhadi. Objaverse: A universe of annotated 3d objects. In *Proceedings of the IEEE/CVF conference on computer vision and pattern recognition*, pages 13142–13153, 2023.
- [5] Miaojie Feng, Junda Cheng, Hao Jia, Longliang Liu, Gangwei Xu, and Xin Yang. Mc-stereo: Multi-peak lookup and cascade search range for stereo matching. In *International Conference on 3D Vision (3DV)*, pages 344–353. IEEE, 2024.
- [6] Adrien Gaidon, Qiao Wang, Yohann Cabon, and Eleonora Vig. Virtual worlds as proxy for multi-object tracking analysis. In *Proceedings of the IEEE/CVF Conference on Computer Vision and Pattern Recognition*, pages 4340–4349, 2016.
- [7] Andreas Geiger, Philip Lenz, and Raquel Urtasun. Are we ready for autonomous driving? the kitti vision benchmark suite. In *Proceedings of the IEEE/CVF Conference on Computer Vision and Pattern Recognition*, 2012.
- [8] Tongfan Guan, Chen Wang, and Yun-Hui Liu. Neural markov random field for stereo matching. In *Proceedings of the IEEE/CVF Conference on Computer Vision and Pattern Recognition*, pages 5459–5469, 2024.
- [9] Jiankun Li, Peisen Wang, Pengfei Xiong, Tao Cai, Ziwei Yan, Lei Yang, Jiangyu Liu, Haoqiang Fan, and Shuaicheng Liu. Practical stereo matching via cascaded recurrent network with adaptive correlation. In *Proceedings of the IEEE/CVF Conference on Computer Vision and Pattern Recognition*, pages 16263–16272, 2022.
- [10] Lahav Lipson, Zachary Teed, and Jia Deng. Raft-stereo: Multilevel recurrent field transforms for stereo matching. In *International Conference on 3D Vision (3DV)*, pages 218–227. IEEE, 2021.
- [11] Nikolaus Mayer, Eddy Ilg, Philip Hausser, Philipp Fischer, Daniel Cremers, Alexey Dosovitskiy, and Thomas Brox. A large dataset to train convolutional networks for disparity, optical flow, and scene flow estimation. In *Proceedings of the IEEE/CVF Conference on Computer Vision and Pattern Recognition*, pages 4040–4048, 2016.
- [12] Moritz Menze and Andreas Geiger. Object scene flow for autonomous vehicles. In *Proceedings of the IEEE/CVF Conference on Computer Vision and Pattern Recognition*, pages 3061–3070, 2015.
- [13] Adam Paszke, Sam Gross, Francisco Massa, Adam Lerer, James Bradbury, Gregory Chanan, Trevor Killeen, Zeming Lin, Natalia Gimelshein, Luca Antiga, et al. Pytorch: An imperative style, high-performance deep learning library. *Advances in neural information processing systems*, 32, 2019.
- [14] Daniel Scharstein, Heiko Hirschmüller, York Kitajima, Greg Krathwohl, Nera Nešić, Xi Wang, and Porter Westling. High-resolution stereo datasets with subpixel-accurate ground truth. In *Pattern Recognition: 36th German Conference, GCPR 2014, Münster, Germany, September 2-5, 2014, Proceedings 36*, pages 31–42. Springer, 2014.
- [15] Thomas Schops, Johannes L Schonberger, Silvano Galliani, Torsten Sattler, Konrad Schindler, Marc Pollefeys, and Andreas Geiger. A multi-view stereo benchmark with high-resolution images and multi-camera videos. In *Proceedings of the IEEE/CVF Conference on Computer Vision and Pattern Recognition*, pages 3260–3269, 2017.
- [16] Fabio Tosi, Yiyi Liao, Carolin Schmitt, and Andreas Geiger. Smd-nets: Stereo mixture density networks. In *Proceedings of the IEEE/CVF Conference on Computer Vision and Pattern Recognition*, pages 8942–8952, 2021.
- [17] Jonathan Tremblay, Thang To, and Stan Birchfield. Falling things: A synthetic dataset for 3d object detection and pose estimation. In *Proceedings of the IEEE/CVF Conference on Computer Vision and Pattern Recognition Workshops*, pages 2038–2041, 2018.
- [18] Qiang Wang, Shizhen Zheng, Qingsong Yan, Fei Deng, Kaiyong Zhao, and Xiaowen Chu. Irs: A large naturalistic indoor robotics stereo dataset to train deep models for disparity and surface normal estimation. In *IEEE International Conference on Multimedia and Expo (ICME)*, pages 1–6. IEEE, 2021.
- [19] Wenshan Wang, Delong Zhu, Xiangwei Wang, Yaoyu Hu, Yuheng Qiu, Chen Wang, Yafei Hu, Ashish Kapoor, and Sebastian Scherer. Tartanair: A dataset to push the limits of visual slam. In *IEEE/RSJ International Conference on Intelligent Robots and Systems (IROS)*, pages 4909–4916. IEEE, 2020.
- [20] Xianqi Wang, Gangwei Xu, Hao Jia, and Xin Yang. Selective-stereo: Adaptive frequency information selection for stereo matching. In *Proceedings of the IEEE/CVF Conference on Computer Vision and Pattern Recognition*, pages 19701–19710, 2024.
- [21] Zhou Wang, Alan C. Bovik, Hamid R. Sheikh, and Eero P. Simoncelli. Image quality assessment: From error visibility to structural similarity. *IEEE Transactions on Image Processing*, 13(4):600–612, 2004.
- [22] Philippe Weinzaepfel, Thomas Lucas, Vincent Leroy, Yohann Cabon, Vaibhav Arora, Romain Brégier, Gabriela Csurka, Leonid Antsfeld, Boris Chidlovskii, and Jérôme Revaud. Croco v2: Improved cross-view completion pre-training for stereo matching and optical flow. In *Proceedings of the IEEE/CVF International Conference on Computer Vision*, pages 17969–17980, 2023.

- [23] Bowen Wen, Matthew Trepte, Joseph Aribido, Jan Kautz, Orazio Gallo, and Stan Birchfield. Foundationstereo: Zero-shot stereo matching. In *Proceedings of the Computer Vision and Pattern Recognition Conference*, pages 5249–5260, 2025.
- [24] Bin Xu, Yuhua Xu, Xiaoli Yang, Wei Jia, and Yulan Guo. Bilateral grid learning for stereo matching networks. In *Proceedings of the IEEE/CVF conference on computer vision and pattern recognition*, pages 12497–12506, 2021.
- [25] Gangwei Xu, Xianqi Wang, Xiaohuan Ding, and Xin Yang. Iterative geometry encoding volume for stereo matching. In *Proceedings of the IEEE/CVF conference on computer vision and pattern recognition*, pages 21919–21928, 2023.
- [26] Gangwei Xu, Yun Wang, Junda Cheng, Jinhui Tang, and Xin Yang. Accurate and efficient stereo matching via attention concatenation volume. *IEEE Transactions on Pattern Analysis and Machine Intelligence*, 46(4):2461–2474, 2023.
- [27] Haofei Xu, Jing Zhang, Jianfei Cai, Hamid Rezatofighi, Fisher Yu, Dacheng Tao, and Andreas Geiger. Unifying flow, stereo and depth estimation. *IEEE Transactions on Pattern Analysis and Machine Intelligence*, 2023.
- [28] Guorun Yang, Xiao Song, Chaoqin Huang, Zhidong Deng, Jianping Shi, and Bolei Zhou. Drivingstereo: A large-scale dataset for stereo matching in autonomous driving scenarios. In *Proceedings of the IEEE/CVF Conference on Computer Vision and Pattern Recognition*, pages 899–908, 2019.
- [29] Jiawei Zhang, Jiahe Li, Lei Huang, Xiaohan Yu, Lin Gu, Jin Zheng, and Xiao Bai. Robust synthetic-to-real transfer for stereo matching. In *Proceedings of the IEEE/CVF Conference on Computer Vision and Pattern Recognition*, pages 20247–20257, 2024.
